# Supplementary material for: SemVLP: Vision-Language Pre-training by Aligning Semantics at Multiple Levels
Source: arXiv:2103.07829 source file (2021-03-14)
Supplement: Supplementary file 1 [file naacl2021.tex]

% This must be in the first 5 lines to tell arXiv to use pdfLaTeX, which is strongly recommended.
\pdfoutput=1
% In particular, the hyperref package requires pdfLaTeX in order to break URLs across lines.

\documentclass[11pt]{article}

% Remove the "review" option to generate the final version.
\usepackage{naacl2021}

% Standard package includes
\usepackage{times}
\usepackage{latexsym}

% For proper rendering and hyphenation of words containing Latin characters (including in bib files)
\usepackage[T1]{fontenc}
% For Vietnamese characters
% \usepackage[T5]{fontenc}
% See https://www.latex-project.org/help/documentation/encguide.pdf for other character sets

% This assumes your files are encoded as UTF8
\usepackage[utf8]{inputenc}

% This is not strictly necessary, and may be commented out,
% but it will improve the layout of the manuscript,
% and will typically save some space.
\usepackage{microtype}

% If the title and author information does not fit in the area allocated, uncomment the following
%
%\setlength\titlebox{<dim>}
%
% and set <dim> to something 5cm or larger.

\title{Supplementary material}

% Author information can be set in various styles:
% For several authors from the same institution:
% \author{Author 1 \and ... \and Author n \\
%         Address line \\ ... \\ Address line}
% if the names do not fit well on one line use
%         Author 1 \\ {\bf Author 2} \\ ... \\ {\bf Author n} \\
% For authors from different institutions:
% \author{Author 1 \\ Address line \\  ... \\ Address line
%         \And  ... \And
%         Author n \\ Address line \\ ... \\ Address line}
% To start a seperate ``row'' of authors use \AND, as in
% \author{Author 1 \\ Address line \\  ... \\ Address line
%         \AND
%         Author 2 \\ Address line \\ ... \\ Address line \And
%         Author 3 \\ Address line \\ ... \\ Address line}

% \author{First Author \\
%   Affiliation / Address line 1 \\
%   Affiliation / Address line 2 \\
%   Affiliation / Address line 3 \\
%   \texttt{email@domain} \\\And
%   Second Author \\
%   Affiliation / Address line 1 \\
%   Affiliation / Address line 2 \\
%   Affiliation / Address line 3 \\
%   \texttt{email@domain} \\}

\begin{document}
\maketitle
\section*{Downstream Tasks}
For all the tasks, We use the architecture mode with the optimal performance on development set for final evaluation. The hidden state of $h^L_{CLS}$ (single-stream mode) or $o^L_{IMG}$ (two-stream mode) is used to measure the cross-modality relevance. 

\subsection{Visual Question Answering (VQA)}
The VQA task requires the model to answer natural language questions given an image. We conduct experiments on the widely-used VQA v2.0 dataset~\citep{antol2015vqa}, which contains 204K images and 1.1M questions about these images. Following~\citep{anderson2018bottom}, we treat VQA as a multi-label classification task by picking an answer from a shared set consisting of 3,129 answers. We use the hidden state of $h^L_{CLS}$ (single-stream mode) or $o^L_{IMG}$ (two-stream mode) to map the representation into 3,129 possible answers with an additional MLP layer. The model is optimized with a binary cross-entropy loss on the soft target scores.
We fine-tune the SemVLP model on the VQA training data for 3 epochs with a batch size of 32, and use the BERT Adam optimizer with an initial learning rate of 5e-5. At inference, a Softmax function is used for prediction.

\subsection{Image-Text Retrieval}
The image-text retrieval task consists of two sub-tasks: image retrieval and text retrieval, depending on which modality is used as the retrieval target. We conduct experiments on the Flickr30K dataset~\citep{young2014image}, which contains 31,000 images collected from Flickr website, each associated with 5 captions. We follow the same split in~\citep{lee2018stacked} for training and evaluation. 

%We sample three pairs of image and text, one positive pair from the dataset and two negative pairs by randomly replacing its sentence/image with others. 
During fine-tuning, we follow the method in UNITER~\citep{chenuniter} and formulate it as a ranking problem. We use the hidden state of $h^L_{CLS}$ (single-stream mode) or $o^L_{IMG}$ (two-stream mode) to compute the similarity scores for the sampled positive and negative pairs, and maximize the margin between them through the circle loss~\citep{sun2020circle} as in ERNIE-Vil~\citep{yu2020ernie}.
We fine-tune our model for 4 epochs with a batch size of 64 and a learning rate of 5e-5. Moreover, we use hard negatives sampling as in~\citep{chenuniter} to further improve the performance.

\subsection{Natural Language Visual Reasoning for Real (NLVR2)}
NLVR2~\citep{suhr2018corpus} is a challenging task for visual reasoning. The goal is to determine whether a natural language statement is true about a pair of images. It consists of 86K/7K/7K data for training/development/test. Since each data example in NLVR2 has two natural images $img_0$, $img_1$ and one language statement $s$, we use SemVLP to encode the two image-statement pairs ($img_0$, $s$) and ($img_1$, $s$), then train a classifier based on the concatenation of the two outputs as in LXMERT~\citep{tan2019lxmert}. We fine-tune SemVLP with a batch size of 32 and a learning rate of 5e-5 for 4 epochs.

\subsection{Visual Reasoning in the Real World (GQA)}
GQA is an image question answering task, which emphasizes on the reasoning capability of the model to answer a question. We conduct experiments on the public GQA 2019 dataset~\citep{hudson2019gqa}.  For each question, the model picks a proper answer from a shared set of 1,852 candidate answers. We follow the two-stage fine-tuning method in OSCAR~\cite{li2020oscar}, where SemVLP model is first fine-tuned on unbalanced ``all-split'' for 2 epochs, and then fine-tune on the ``balanced-split'' for 2 epochs with batch size of 32 and learning rate of 5e-6.

\bibliography{anthology}
\bibliographystyle{acl_natbib}

\end{document}
